# Supplementary material for: What's under the hood: Investigating Automatic Metrics on Meeting Summarization
Source: arXiv:2404.11124 source file (2024-10-18)
Supplement: Supplementary file 1 [file appendix.tex]

\section{Literature Review: Challenges}
\label{sec:appendix_challenges}
% Table generated by Excel2LaTeX from sheet 'Tabelle11'
\begin{table*}[htbp!]
  \centering
  \small
    \begin{tabular}{p{10em}p{35em}}
   % Table generated by Excel2LaTeX from sheet 'Tabelle11'

    \toprule
    Reference & Title \\
    \midrule
    \citet{ KhalifaBM21a} & A Bag of Tricks for Dialogue Summarization   \\
    \midrule
    \citet{AntonyASK23} & A Survey of Advanced Methods for Efficient Text Summarization   \\
    \midrule
    \citet{FengFQ22c} & A Survey on Dialogue Summarization: Recent Advances and New Frontiers   \\
    \midrule
    \citet{RennardSHV23} & Abstractive Meeting Summarization: A Survey   \\
    \midrule
    \citet{ZhangZ21} & Advances in Multi-turn Dialogue Comprehension: A Survey   \\
    \midrule
    \citet{WangZZC22b} & Analyzing and Evaluating Faithfulness in Dialogue Summarization   \\
    \midrule
    \citet{ ZhangNYZ21a} & An Exploratory Study on Long Dialogue Summarization: What Works and What's Next   \\
    \midrule
    \citet{ShindeGSB22} & Automatic Minuting: A Pipeline Method for Generating Minutes from Multi-Party Meeting Proceedings  \\
    \midrule
    \citet{LiHXA23a} & Discourse Structure Extraction from Pre-Trained and Fine-Tuned Language Models in Dialogues  \\
    \midrule
    \citet{ChenDY22a} & Human-in-the-loop Abstractive Dialogue Summarization   \\
    \midrule
    \citet{JacquenetBL19c} & Meeting Summarization, A Challenge for Deep Learning   \\
    \midrule
    \citet{KumarK22d} & Meeting Summarization: A Survey of the State of the Art   \\
    \midrule
    \citet{MaynezNBM20} & On Faithfulness and Factuality in Abstractive Summarization   \\
    \midrule
    \citet{JiaRLZ22} & Taxonomy of Abstractive Dialogue Summarization: Scenarios, Approaches and Future Directions   \\
    \midrule
    \citet{GuTL22} & Who Says What to Whom: A Survey of Multi-Party Conversations  \\
    \midrule
    \citet{MaZEGWS22}&  Multi-document Summarization via Deep Learning Techniques: A Survey \\
    \midrule
    \citet{KoayRDB20d} &  How Domain Terminology Affects Meeting Summarization Performance\\
    \midrule
    \citet{RichardsonH23} &  Commonsense Reasoning for Conversational AI: A Survey of the State of the Art\\
    \bottomrule
    \end{tabular}%
    \caption{Retrieved sources describing challenges relevant for meeting summarization.}
  \label{tab:appendix_challenges}%
\end{table*}%

\Cref{tab:appendix_challenges} shows an overview of the sources considered to define the key challenges in meeting summarization

\section{Literature Review: Errors}
\label{sec:appendix_errors}
\begin{table*}[htbp!]
  \centering
  \scriptsize
    \begin{tabular}{p{10em}p{35em}}
    \toprule
    Reference & Title \\
    \midrule
    \citet{BahrainianZCE22} & CATS: Customizable Abstractive Topic-based Summarization \\ \midrule
    \citet{BertschNG22a} & He Said, She Said: Style Transfer for Shifting the Perspective of Dialogues \\ \midrule
    \citet{ChoDGB21} & StreamHover: Livestream Transcript Summarization and Annotation \\ \midrule
    \citet{ChenDY22a} & Human-in-the-loop Abstractive Dialogue Summarization \\ \midrule
    \citet{FangZCD22a} & From spoken dialogue to formal summary: An utterance rewriting for dialogue summarization \\ \midrule
    \citet{FengFQG21c} & Dialogue Discourse-Aware Graph Model and Data Augmentation for Meeting Summarization \\ \midrule
    \citet{GengZYQ22a} & Improving Abstractive Dialogue Summarization with Speaker-Aware Supervised Contrastive Learning \\ \midrule
    \citet{GhoshalEAL22} & Improving Faithfulness of Abstractive Summarization by Controlling Confounding Effect of Irrelevant Sentences \\ \midrule
    \citet{HuangSMX23} & SWING : Balancing Coverage and Faithfulness for Dialogue Summarization \\ \midrule
    \citet{JoshiCLW20} & SpanBERT: Improving Pre-training by Representing and Predicting Spans \\ \midrule
    \citet{KhalifaBM21a} & A Bag of Tricks for Dialogue Summarization \\ \midrule
    \citet{KoayRDB20d} & How Domain Terminology Affects Meeting Summarization Performance \\ \midrule
    \citet{Li22} & URAMDS: Utterances Relation Aware Model for Dialogue Summarization: A Combined Model for Dialogue Summarization \\ \midrule
    \citet{LiHXA23a} & Discourse Structure Extraction from Pre-Trained and Fine-Tuned Language Models in Dialogues \\ \midrule
    \citet{LiLG23} & Factual Error Correction in Summarization with Retriever-Reader Pipeline \\ \midrule
    \citet{LiZBP22} & Improving Factual Consistency of Dialogue Summarization with Fact-Augmentation Mechanism \\ \midrule
    \citet{LinZXZ23} & Topic-Oriented Dialogue Summarization \\ \midrule
    \citet{LiuC21a} & Dynamic Sliding Window for Meeting Summarization \\ \midrule
    \citet{LiuSC} & Coreference-Aware Dialogue Summarization \\ \midrule
    \citet{LiuWXL19} & Automatic Dialogue Summary Generation for Customer Service \\ \midrule
    \citet{LiuZZC21} & Topic-Aware Contrastive Learning for Abstractive Dialogue Summarization \\ \midrule
    \citet{QiHSL22} & A Knowledge Graph-Based Abstractive Model Integrating Semantic and Structural Information for Summarizing Chinese Meetings \\ \midrule
    \citet{RaviNS23} & COMET-M: Reasoning about Multiple Events in Complex Sentences \\ \midrule
    \citet{SongLWY22} & Towards Abstractive Grounded Summarization of Podcast Transcripts \\ \midrule
    \citet{TangNWW22a} & CONFIT: Toward Faithful Dialogue Summarization with Linguistically-Informed Contrastive Fine-tuning \\ \midrule
    \citet{WangFNM22} & STRUDEL: Structured Dialogue Summarization for Dialogue Comprehension \\ \midrule
    \citet{XieHZL22} & View Dialogue in 2D: A Two-stream Model in Time-speaker Perspective for Dialogue Summarization and beyond \\ \midrule
    \citet{XuTJZ20} & Learning an Effective Context-Response Matching Model with Self-Supervised Tasks for Retrieval-based Dialogues \\ \midrule
    \citet{ZhaoNLH23} & Generation of Coherent Multi-Sentence Texts with a Coherence Mechanism \\ \midrule
    \citet{ZhongYYZ21d} & QMSum: A New Benchmark for Query-based Multi-domain Meeting Summarization \\ \midrule
    \citet{ZhuXZH20c} & A Hierarchical Network for Abstractive Meeting Summarization with Cross-Domain Pretraining \\ \midrule
    \citet{ZouSTF23} & Towards Understanding Omission in Dialogue Summarization \\ \midrule
    \citet{14} & SUMMARIZATION USING NTC APPROACH BASED ON KEYWORD EXTRACTION FOR DISCUSSION FORUMS \\
    \bottomrule
    \end{tabular}%
    \caption{Retrieved sources describing errors relevant for meeting summarization.}
  \label{tab:appendix_errors}%
\end{table*}%

\Cref{tab:appendix_errors} shows an overview of secondary sources considered to define the observable errors in meeting summarization

\begin{table*}[htbp]
  \centering
  \scriptsize
   \begin{tabular}{p{50pt}p{40em}}
    \toprule
    Error Type & \multicolumn{1}{l}{Example} \\
    \midrule
    Missing information & This is the eleventh evidence session on the Children (Abolition of Defence of Reasonable Punishment) Bill. Firstly, Barry Hughes, Chief Crown Prosecutor for Wales, introduced the Children and Young People and Education Bill. The Bill was introduced in 2007. It was aimed at addressing the divergence between the criminal law in Wales and England and the CPS guidelines. Secondly, the Bill was designed to address the public interest in criminal law. The bill was designed for the purpose of reducing the number of criminal charges and to make it more relevant to the criminal justice system.\newline{} (Comment by authors: \color{red} Six main topics had been discussed\color{black}.) \\
    \midrule
    Redundancy & This was the first detailed design meeting of the remote control. Industrial Designer, User Interface, \color{red}Industrial Designer and Industrial Designer \color{black} presented the prototype. User Interface gave a presentation on the technical aspects of remote control design. Then Industrial Designer gave the final prototype presentation. After that, the team discussed the cost of the new remote control, which was twelve fifty Euros. Finally, the group discussed the technical features of the product, such as the shape of the buttons, the size of the LCD screen, the colour of the screen, and the size and shape. Lastly, the project manager gave a detailed design review of the project. \\
    \midrule
    Wrong references & The meeting was mainly about the functional design of the remote control. \color{red} Industrial Designer \color{black} presented the technical function design for user interface, User Interface designer presented user interface design, \color{red} Marketing \color{black} presented  User Interface design, and \color{red} Marketing \color{black} presented the industrial design. The industrial design was simple and easy to use. The user interface designer presented the user interface concept. The \color{red} User Interface \color{black} Designer presented a presentation on the technical functions design for remote control, and the \color{red} Industrial Designer \color{black} gave the presentation on user interface. The group then discussed the product requirements and the cost of the product.\newline{}Finally, the group decided to design a wireless remote control based on the current market trends. \\
    \midrule
    Incorrect reasoning & The group discussed the conceptual model of the remote control. Industrial Designer and User Interface gave a presentation on the conceptual design. Then, Project Manager gave a brief discussion on the cost of the new remote control and suggested that it should be simple and easy to use. The group also discussed the design of the LCD screen and the shape of the buttons. Finally, the group decided that they should make the LCD display with a scroll wheel on the side and the back-lights b on the top of it.\newline{}(Comment by the authors: \color{red} The meeting was about the functional design\color{black}.) \\
    \midrule
    Hallucination & The Children, Young People and Education Committee \color{red} (M\&E) \color{black} is an inquiry on education otherwise than at school. The meeting was mainly focused on the impact of the new curriculum on EOTAS learners. The committee also discussed the challenges faced by the local authorities in terms of providing support and support to young people who are at risk of being excluded. In particular, the committee discussed the difficulties faced by students who were excluded from mainstream education, and how to deal with them. In addition, the meeting discussed the impact on the children who are excluded and how they should be treated.\newline{}(Comment by the authors: M\&E is not an abbreviation mentioned during the meeting.) \\
    \midrule
    Incoherence & The meeting was mainly about the functional design of the remote control. \color{red} Industrial Designer presented the technical function design for user interface, User Interface designer presented user interface design, Marketing presented User Interface design, and Marketing presented the industrial design. The industrial design was simple and easy to use. The user interface designer presented the user interface concept. The User Interface Designer presented a presentation on the technical functions design for remote control, and the Industrial Designer gave the presentation on user interface. \color{black} The group then discussed the product requirements and the cost of the product. Finally, the group decided to design a wireless remote control based on the current market trends. \\
    \midrule
    Linguistic inaccuracy & The meeting was mainly about the reorganization of the Meeting Recorder data. The transcribers were working on a new version of the transcriptions. The team was working on the new version and the team was looking for a way to make it easier to transcribe and to use them for training a \color{red} (disfmarker) \color{black} or a non-pre- segmented version. The meeting ended with the transcriber meeting and a discussion about the team's progress. The group agreed that they would be able to improve the recording rate.\newline{}They also agreed that recording would be a good thing to do. \\
    \midrule
    Structural disorganization & The meeting began with a discussion about the meeting format. \color{red} The meeting ended \color{black} with a presentation of the Meeting Recording project.\newline{}The group discussed how they could use the Meeting Recorder to record the meeting. Then, the group discussed the data from Broadcast News.\newline{} \color{red} Finally \color{black}, the meeting concluded with the group discussing how they would use the meeting data. The team also discussed the possibility of adding more microphones to the meeting, which would be useful for summarization. Lastly, the team discussed the topic of the recording of the meeting in order to better understand the participants' speech. \\
    \bottomrule
    \end{tabular}%
      \caption{Selection of summary predictions drawn from all three models. We picked the clearest examples for demonstration purpose.}
  \label{tab:error_Type_examples}%
\end{table*}%

\Cref{tab:error_Type_examples} provides examples of observed error types.

\section{Analysis: Correlation and Significance Matrices}
\label{sec:appendix_corr_sig_matrices}
\input{}
\Cref{missing} and \Cref{missing} show the Point-biserial correlation matrices between each challenge and each observable error for encoder-decoder and autoregressive models respectively.
The corresponding significance matrices are in \Cref{missing} and \Cref{missing}.
The significance matrices for \Cref{tab:correlation_metric_error} from RQ1 and \Cref{tab:correlation_metric_error_impact} from RQ3 are presented in \Cref{missing} and \Cref{missing} respectively.

\section{Analysis: Manual Inspection}
\label{sec:appendix_manual_inspection}
\begin{table*}[h]
\centering
\scriptsize
\begin{tabular}{p{10mm}p{95mm}p{25mm}p{14mm}}
\toprule
\textbf{Metrics failing} & \textbf{Transcript} & \textbf{Metric Scores} & \textbf{Present \newline Errors}\\
% \midrule
% few & The meeting was mainly about the functional design of the remote control.
% Industrial Designer presented the technical function design for user interface, User Interface designer presented user interface design, Marketing presented User Interface design, and Marketing presented the industrial design.
% The industrial design was simple and easy to use.
% The user interface designer presented the user interface concept.
% The User Interface Designer presented a presentation on the technical functions design for remote control, and the Industrial Designer gave the presentation on user interface.
% The group then discussed the product requirements and the cost of the product.
% Finally, the group decided to design a wireless remote control based on the current market trends. & 
% Rouge1: 0.49 \newline
% Rouge2: 0.23 \newline
% RougeL: 0.29 \newline
% BertScore: 0.329 \newline
% BLEU: 0.115 \newline
% PPL: 18.0 \newline
% METEOR: 0.34 \newline
% BLANC: 0.11 \newline
% LENS: 53.0 \newline
% QuestEval: 0.17 &
% MI (low) \newline
% Red (mid) \newline
% WR (high) \newline
% Hal ? \\
\midrule
most & The meeting began with a discussion about the recording of the meeting.
The meeting ended with a presentation by the team members on the progress of the recording.
The team members then discussed the process of recording the meeting, and how they could make it easier for people to access the transcriptions.
Finally, the team discussed how to make the recording easier and more efficient.
They also discussed the possibility of having a printout of the transcript, which would be easier to transcribe, and the possibility that the transcript could be edited by hand.
Lastly, they discussed the technical aspects of recording. & 
Rouge1: 0.49 \newline
Rouge2: 0.23 \newline
RougeL: 0.29 \newline
BertScore: 0.329 \newline
BLEU: 0.115 \newline
PPL: 18.0 \newline
METEOR: 0.34 \newline
BLANC: 0.11 \newline
LENS: 53.0 \newline
QuestEval: 0.17 &
MI (low) \newline
Red (mid) \newline
WR (high) \newline
Hal (low) \newline
SD (low) \\
\midrule
none & The group discussed the working design of the remote control.
Industrial Designer, User Interface, Marketing, Industrial Designer and Industrial Designer gave a presentation on the design of remote controls.
They talked about the basic functions, like buttons, volume, channels, etcetera.
They also talked about how they could make it more like a mobile phone.
Then, they discussed how to make it look and feel like a remote control for the elderly people.
Finally, they talked about their personal preferences.
They decided to use standard buttons instead of the standard ones.
The group decided to make a new remote control with a simple design. & 
Rouge1: 0.49 \newline
Rouge2: 0.23 \newline
RougeL: 0.29 \newline
BertScore: 0.329 \newline
BLEU: 0.115 \newline
PPL: 18.0 \newline
METEOR: 0.34 \newline
BLANC: 0.11 \newline
LENS: 53.0 \newline
QuestEval: 0.17 &
MI (low) \newline
Red (mid) \newline
WR (high) \newline
Hal ? \\
\bottomrule
\end{tabular}
\caption{Example of automatic metrics reacting to different summaries with varying degree of reaction. Human annotated errors and impact scores are presented for reference. Score of 1 means low impact, score of 5 is a high impact.}
\label{tab:human_annotation}
\end{table*}
We manually inspected the human annotations (see \Cref{sec:human_annotation}) and related metric scores and display a representative selection in \Cref{tab:human_annotation}.
Both examples show metrics presenting errors annotated by our expert evaluators.
The first row shows a summary with some missing information such as XY, structural disorganization and hallucination, mid redundancy and high wrong referenciation.
These errors result in a summary with a limited picture of the overall meeting.
Despite these shortcomings, the scores are among the highest of observed scores.
The second row shows a summary for a transcript from the same dataset subset (AMI), with a comparable set of errors and severities and a similar limited summary.
However, this time the metrics better reflect the quality of the summary, especially the scores XY.
Judging from the observed errors, the low values of XY are expected as described in RQ1.

Results presented in this section highlight the different reactions of automatic metrics compared to human annotations.

\section{Inner Annotator Agreement: Breakdown of scores}
>> Table X provides the inner annotator scores broken down for each individual model

\section{Metrics: Details on the evaluation metrics used}
>> Table X provides additional details on the metric versions and the parameters used.
