# Supplementary material for: What's under the hood: Investigating Automatic Metrics on Meeting Summarization
Source: arXiv:2404.11124 source file (2024-10-18)
Supplement: Supplementary file 2 [file Error_examples.tex]

\begin{table*}[htbp]
  \centering
  \scriptsize
   \begin{tabular}{p{50pt}p{40em}}
    \toprule
    Error Type & \multicolumn{1}{l}{Example} \\
    \midrule
    Missing information & This is the eleventh evidence session on the Children (Abolition of Defence of Reasonable Punishment) Bill. Firstly, Barry Hughes, Chief Crown Prosecutor for Wales, introduced the Children and Young People and Education Bill. The Bill was introduced in 2007. It was aimed at addressing the divergence between the criminal law in Wales and England and the CPS guidelines. Secondly, the Bill was designed to address the public interest in criminal law. The bill was designed for the purpose of reducing the number of criminal charges and to make it more relevant to the criminal justice system.\newline{} (Comment by authors: \color{red} Six main topics had been discussed\color{black}.) \\
    \midrule
    Redundancy & This was the first detailed design meeting of the remote control. Industrial Designer, User Interface, \color{red}Industrial Designer and Industrial Designer \color{black} presented the prototype. User Interface gave a presentation on the technical aspects of remote control design. Then Industrial Designer gave the final prototype presentation. After that, the team discussed the cost of the new remote control, which was twelve fifty Euros. Finally, the group discussed the technical features of the product, such as the shape of the buttons, the size of the LCD screen, the colour of the screen, and the size and shape. Lastly, the project manager gave a detailed design review of the project. \\
    \midrule
    Wrong references & The meeting was mainly about the functional design of the remote control. \color{red} Industrial Designer \color{black} presented the technical function design for user interface, User Interface designer presented user interface design, \color{red} Marketing \color{black} presented  User Interface design, and \color{red} Marketing \color{black} presented the industrial design. The industrial design was simple and easy to use. The user interface designer presented the user interface concept. The \color{red} User Interface \color{black} Designer presented a presentation on the technical functions design for remote control, and the \color{red} Industrial Designer \color{black} gave the presentation on user interface. The group then discussed the product requirements and the cost of the product.\newline{}Finally, the group decided to design a wireless remote control based on the current market trends. \\
    \midrule
    Incorrect reasoning & The group discussed the conceptual model of the remote control. Industrial Designer and User Interface gave a presentation on the conceptual design. Then, Project Manager gave a brief discussion on the cost of the new remote control and suggested that it should be simple and easy to use. The group also discussed the design of the LCD screen and the shape of the buttons. Finally, the group decided that they should make the LCD display with a scroll wheel on the side and the back-lights b on the top of it.\newline{}(Comment by the authors: \color{red} The meeting was about the functional design\color{black}.) \\
    \midrule
    Hallucination & The Children, Young People and Education Committee \color{red} (M\&E) \color{black} is an inquiry on education otherwise than at school. The meeting was mainly focused on the impact of the new curriculum on EOTAS learners. The committee also discussed the challenges faced by the local authorities in terms of providing support and support to young people who are at risk of being excluded. In particular, the committee discussed the difficulties faced by students who were excluded from mainstream education, and how to deal with them. In addition, the meeting discussed the impact on the children who are excluded and how they should be treated.\newline{}(Comment by the authors: M\&E is not an abbreviation mentioned during the meeting.) \\
    \midrule
    Incoherence & The meeting was mainly about the functional design of the remote control. \color{red} Industrial Designer presented the technical function design for user interface, User Interface designer presented user interface design, Marketing presented User Interface design, and Marketing presented the industrial design. The industrial design was simple and easy to use. The user interface designer presented the user interface concept. The User Interface Designer presented a presentation on the technical functions design for remote control, and the Industrial Designer gave the presentation on user interface. \color{black} The group then discussed the product requirements and the cost of the product. Finally, the group decided to design a wireless remote control based on the current market trends. \\
    \midrule
    Linguistic inaccuracy & The meeting was mainly about the reorganization of the Meeting Recorder data. The transcribers were working on a new version of the transcriptions. The team was working on the new version and the team was looking for a way to make it easier to transcribe and to use them for training a \color{red} (disfmarker) \color{black} or a non-pre- segmented version. The meeting ended with the transcriber meeting and a discussion about the team's progress. The group agreed that they would be able to improve the recording rate.\newline{}They also agreed that recording would be a good thing to do. \\
    \midrule
    Structural disorganization & The meeting began with a discussion about the meeting format. \color{red} The meeting ended \color{black} with a presentation of the Meeting Recording project.\newline{}The group discussed how they could use the Meeting Recorder to record the meeting. Then, the group discussed the data from Broadcast News.\newline{} \color{red} Finally \color{black}, the meeting concluded with the group discussing how they would use the meeting data. The team also discussed the possibility of adding more microphones to the meeting, which would be useful for summarization. Lastly, the team discussed the topic of the recording of the meeting in order to better understand the participants' speech. \\
    \bottomrule
    \end{tabular}%
      \caption{Selection of summary predictions drawn from all three models. We picked the clearest examples for demonstration purpose.}
  \label{tab:error_Type_examples}%
\end{table*}%
