# Supplementary material for: What's under the hood: Investigating Automatic Metrics on Meeting Summarization
Source: arXiv:2404.11124 source file (2024-10-18)
Supplement: Supplementary file 3 [file appendix_challenges.tex]

% Table generated by Excel2LaTeX from sheet 'Tabelle11'
\begin{table*}[htbp!]
  \centering
  \small
    \begin{tabular}{p{10em}p{35em}}
   % Table generated by Excel2LaTeX from sheet 'Tabelle11'

    \toprule
    Reference & Title \\
    \midrule
    \citet{ KhalifaBM21a} & A Bag of Tricks for Dialogue Summarization   \\
    \midrule
    \citet{AntonyASK23} & A Survey of Advanced Methods for Efficient Text Summarization   \\
    \midrule
    \citet{FengFQ22c} & A Survey on Dialogue Summarization: Recent Advances and New Frontiers   \\
    \midrule
    \citet{RennardSHV23} & Abstractive Meeting Summarization: A Survey   \\
    \midrule
    \citet{ZhangZ21} & Advances in Multi-turn Dialogue Comprehension: A Survey   \\
    \midrule
    \citet{WangZZC22b} & Analyzing and Evaluating Faithfulness in Dialogue Summarization   \\
    \midrule
    \citet{ ZhangNYZ21a} & An Exploratory Study on Long Dialogue Summarization: What Works and What's Next   \\
    \midrule
    \citet{ShindeGSB22} & Automatic Minuting: A Pipeline Method for Generating Minutes from Multi-Party Meeting Proceedings  \\
    \midrule
    \citet{LiHXA23a} & Discourse Structure Extraction from Pre-Trained and Fine-Tuned Language Models in Dialogues  \\
    \midrule
    \citet{ChenDY22a} & Human-in-the-loop Abstractive Dialogue Summarization   \\
    \midrule
    \citet{JacquenetBL19c} & Meeting Summarization, A Challenge for Deep Learning   \\
    \midrule
    \citet{KumarK22d} & Meeting Summarization: A Survey of the State of the Art   \\
    \midrule
    \citet{MaynezNBM20} & On Faithfulness and Factuality in Abstractive Summarization   \\
    \midrule
    \citet{JiaRLZ22} & Taxonomy of Abstractive Dialogue Summarization: Scenarios, Approaches and Future Directions   \\
    \midrule
    \citet{GuTL22} & Who Says What to Whom: A Survey of Multi-Party Conversations  \\
    \midrule
    \citet{MaZEGWS22}&  Multi-document Summarization via Deep Learning Techniques: A Survey \\
    \midrule
    \citet{KoayRDB20d} &  How Domain Terminology Affects Meeting Summarization Performance\\
    \midrule
    \citet{RichardsonH23} &  Commonsense Reasoning for Conversational AI: A Survey of the State of the Art\\
    \bottomrule
    \end{tabular}%
    \caption{Retrieved sources describing challenges relevant for meeting summarization.}
  \label{tab:appendix_challenges}%
\end{table*}%
