# Supplementary material for: What's under the hood: Investigating Automatic Metrics on Meeting Summarization
Source: arXiv:2404.11124 source file (2024-10-18)
Supplement: Supplementary file 4 [file appendix_errors.tex]

\begin{table*}[htbp!]
  \centering
  \scriptsize
    \begin{tabular}{p{10em}p{35em}}
    \toprule
    Reference & Title \\
    \midrule
    \citet{BahrainianZCE22} & CATS: Customizable Abstractive Topic-based Summarization \\ \midrule
    \citet{BertschNG22a} & He Said, She Said: Style Transfer for Shifting the Perspective of Dialogues \\ \midrule
    \citet{ChoDGB21} & StreamHover: Livestream Transcript Summarization and Annotation \\ \midrule
    \citet{ChenDY22a} & Human-in-the-loop Abstractive Dialogue Summarization \\ \midrule
    \citet{FangZCD22a} & From spoken dialogue to formal summary: An utterance rewriting for dialogue summarization \\ \midrule
    \citet{FengFQG21c} & Dialogue Discourse-Aware Graph Model and Data Augmentation for Meeting Summarization \\ \midrule
    \citet{GengZYQ22a} & Improving Abstractive Dialogue Summarization with Speaker-Aware Supervised Contrastive Learning \\ \midrule
    \citet{GhoshalEAL22} & Improving Faithfulness of Abstractive Summarization by Controlling Confounding Effect of Irrelevant Sentences \\ \midrule
    \citet{HuangSMX23} & SWING : Balancing Coverage and Faithfulness for Dialogue Summarization \\ \midrule
    \citet{JoshiCLW20} & SpanBERT: Improving Pre-training by Representing and Predicting Spans \\ \midrule
    \citet{KhalifaBM21a} & A Bag of Tricks for Dialogue Summarization \\ \midrule
    \citet{KoayRDB20d} & How Domain Terminology Affects Meeting Summarization Performance \\ \midrule
    \citet{Li22} & URAMDS: Utterances Relation Aware Model for Dialogue Summarization: A Combined Model for Dialogue Summarization \\ \midrule
    \citet{LiHXA23a} & Discourse Structure Extraction from Pre-Trained and Fine-Tuned Language Models in Dialogues \\ \midrule
    \citet{LiLG23} & Factual Error Correction in Summarization with Retriever-Reader Pipeline \\ \midrule
    \citet{LiZBP22} & Improving Factual Consistency of Dialogue Summarization with Fact-Augmentation Mechanism \\ \midrule
    \citet{LinZXZ23} & Topic-Oriented Dialogue Summarization \\ \midrule
    \citet{LiuC21a} & Dynamic Sliding Window for Meeting Summarization \\ \midrule
    \citet{LiuSC} & Coreference-Aware Dialogue Summarization \\ \midrule
    \citet{LiuWXL19} & Automatic Dialogue Summary Generation for Customer Service \\ \midrule
    \citet{LiuZZC21} & Topic-Aware Contrastive Learning for Abstractive Dialogue Summarization \\ \midrule
    \citet{QiHSL22} & A Knowledge Graph-Based Abstractive Model Integrating Semantic and Structural Information for Summarizing Chinese Meetings \\ \midrule
    \citet{RaviNS23} & COMET-M: Reasoning about Multiple Events in Complex Sentences \\ \midrule
    \citet{SongLWY22} & Towards Abstractive Grounded Summarization of Podcast Transcripts \\ \midrule
    \citet{TangNWW22a} & CONFIT: Toward Faithful Dialogue Summarization with Linguistically-Informed Contrastive Fine-tuning \\ \midrule
    \citet{WangFNM22} & STRUDEL: Structured Dialogue Summarization for Dialogue Comprehension \\ \midrule
    \citet{XieHZL22} & View Dialogue in 2D: A Two-stream Model in Time-speaker Perspective for Dialogue Summarization and beyond \\ \midrule
    \citet{XuTJZ20} & Learning an Effective Context-Response Matching Model with Self-Supervised Tasks for Retrieval-based Dialogues \\ \midrule
    \citet{ZhaoNLH23} & Generation of Coherent Multi-Sentence Texts with a Coherence Mechanism \\ \midrule
    \citet{ZhongYYZ21d} & QMSum: A New Benchmark for Query-based Multi-domain Meeting Summarization \\ \midrule
    \citet{ZhuXZH20c} & A Hierarchical Network for Abstractive Meeting Summarization with Cross-Domain Pretraining \\ \midrule
    \citet{ZouSTF23} & Towards Understanding Omission in Dialogue Summarization \\ \midrule
    \citet{14} & SUMMARIZATION USING NTC APPROACH BASED ON KEYWORD EXTRACTION FOR DISCUSSION FORUMS \\
    \bottomrule
    \end{tabular}%
    \caption{Retrieved sources describing errors relevant for meeting summarization.}
  \label{tab:appendix_errors}%
\end{table*}%
